# Supplementary material for: Globally Minimal Defensive Alliances: A Parameterized Perspective
Source: arXiv:2202.02010 source file (2022-02-04)
Supplement: Supplementary file 1 [file appendix.tex]

\section{Illustration of the reduction in the proof of Theorem 2}
\includegraphics[scale=0.7]{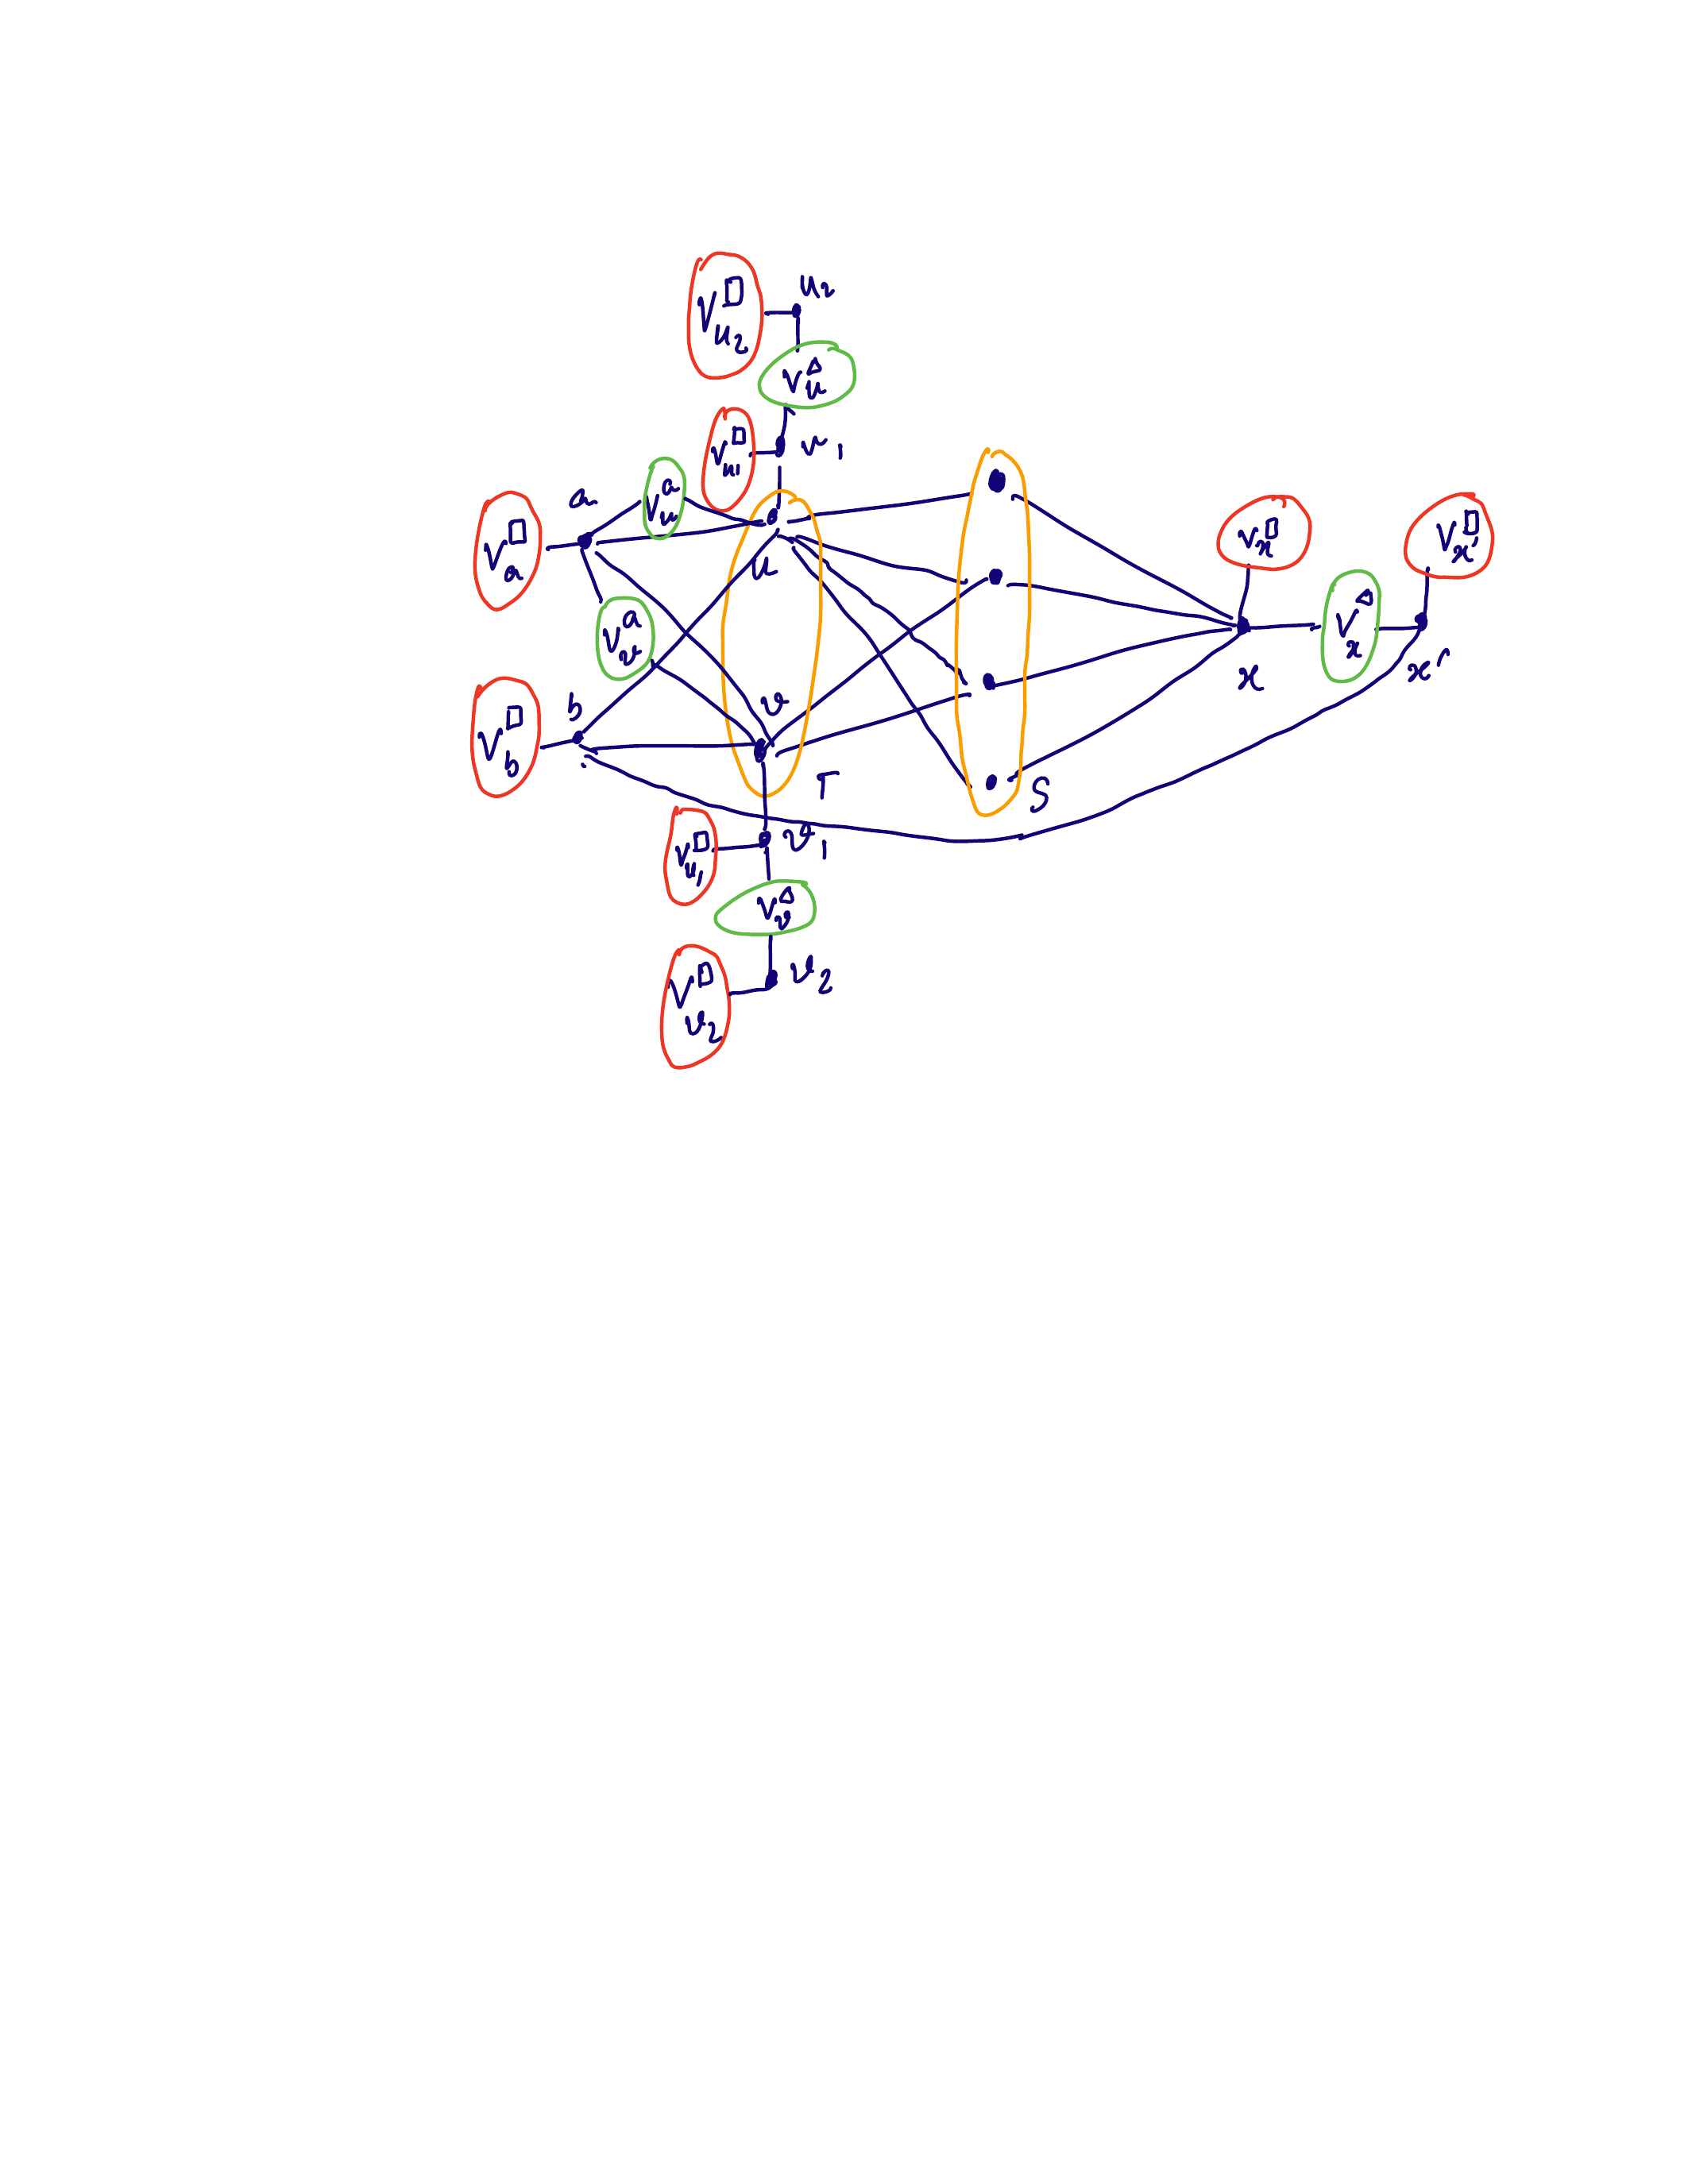}
